# Supplementary material for: Seed Optimization with Frozen Generator for Superior Zero-shot Low-light Enhancement
Source: arXiv:2402.09694 source file (2024-02-15)
Supplement: Supplementary file 1 [file X_suppl.tex]

\clearpage
\setcounter{page}{1}
\maketitlesupplementary
\setcounter{section}{0}

In the accompanying supplementary material, we delve deeper with additional experiments, systematically organized into four sections. Section A expounds on the underlying motivations of our approach, providing more detailed comparisons. Section B scrutinizes the influence of pre-trained weights on performance metrics, The robustness of our method to different generators is demonstrated. Section C examines the effects of loss priors on our model's efficacy. Finally, Section D presents an extensive array of visual comparisons, further elucidating the practical advantages of our proposed method.

\section{More details about Motivation}
$\indent$ In sec \ref{ssec:movitation}, we found that pre-training weights can have a positive effect on model performance, but this effect will disappear as the model parameters are optimized. In fact, we can often observe that the critical point where the effect of the pre-trained model disappears is accompanied by a drastic change in the results of an enhancement. Beyond this juncture, we observe a tendency towards lower contrast and disordered structural features in the reconstruction results.

Figure \ref{fig:supp_optim} illustrates the substantial degradation of pre-training knowledge at this critical point. The comparative analysis of images pre- and post-critical point underscores their suboptimal quality, prompting us to explore alternative strategies for leveraging pre-training knowledge effectively.

\section{Impact of pre-trained weights}
$\indent$To further demonstrate the generalization capabilities of our framework with diverse generative models. We conducted a comparative analysis featuring four prominent generative methods: DCGAN on ImageNet-1K, EAGAN on ImageNet-1K, VAE on COCO, and VQ-VAE-2 on a combined dataset of ImageNet and FFHQ. The evaluation focused on visual performance, utilizing the LOL test dataset for a comprehensive assessment. 
\begin{table}[h]
\centering
\resizebox{\columnwidth}{!}{
\begin{tabular}{lcccc}
\hline
\multicolumn{1}{c}{Method} & DCGAN       & EAGAN    & VAE     & VQVAE-2       \\ \hline
Dataset                    & Imagenet-1K & Imagenet-1K & COCO    & Imagenet+FFHQ \\
PSNR↑                       & 16.09       & 16.94    & 17.19   & 18.10         \\
SSIM↓                       & 0.69        & 0.74     & 0.72    & 0.75          \\
Iteration                  & 4000        & 3000     & 5000    & 2500          \\
Runtime                    & 0.06259     & 0.18580  & 0.01035 & 0.00813       \\
Totaltime                  & 250.8       & 557.4    & 51.75   & 20.3       \\ \hline
\end{tabular}
}
\caption{Training details and effects used by different pretrained generators.}
\label{supp:tab:pretrain}
\end{table}

As shown in Figure~\ref{fig:supp_pretrains}, Generators derived from pre-trained GANs tend to produce images with lower contrast, yet they effectively mitigate color bias. In contrast, generators from pre-trained VAEs are inclined to yield brighter images. Overall, our results demonstrate that various generators can be effectively integrated into our proposed low-light enhancement method, each contributing to substantial improvements in image quality under low-light conditions.

\section{Impact of different losses}
$\indent$ Different priors are used to constrain our model. The figure below shows the role of different loss combinations in the Retinex decomposition process.
\begin{table}[h]
\centering
\resizebox{0.5\columnwidth}{!}{
\begin{tabular}{lc}
\hline
\multicolumn{1}{c}{Method} &Time   \\ \hline
$\mathcal{L}_S$                   & 1.548s \\
$\mathcal{L}_E$                       & 0.194s \\
$\mathcal{L}_{RE}$                       & 0.254s \\
$\mathcal{L}_I$                       & 0.155s \\
other process              & 18.174 \\
totaltime                  & 20.325 \\ \hline
\end{tabular}
}
\caption{Analysis of the time occupied by each loss during the execution of the proposed method.}
\label{supp:tab:time}
\end{table}

\begin{figure*}[t]
    \centering
    \vspace{-0.3cm}
    \includegraphics[width=\linewidth]{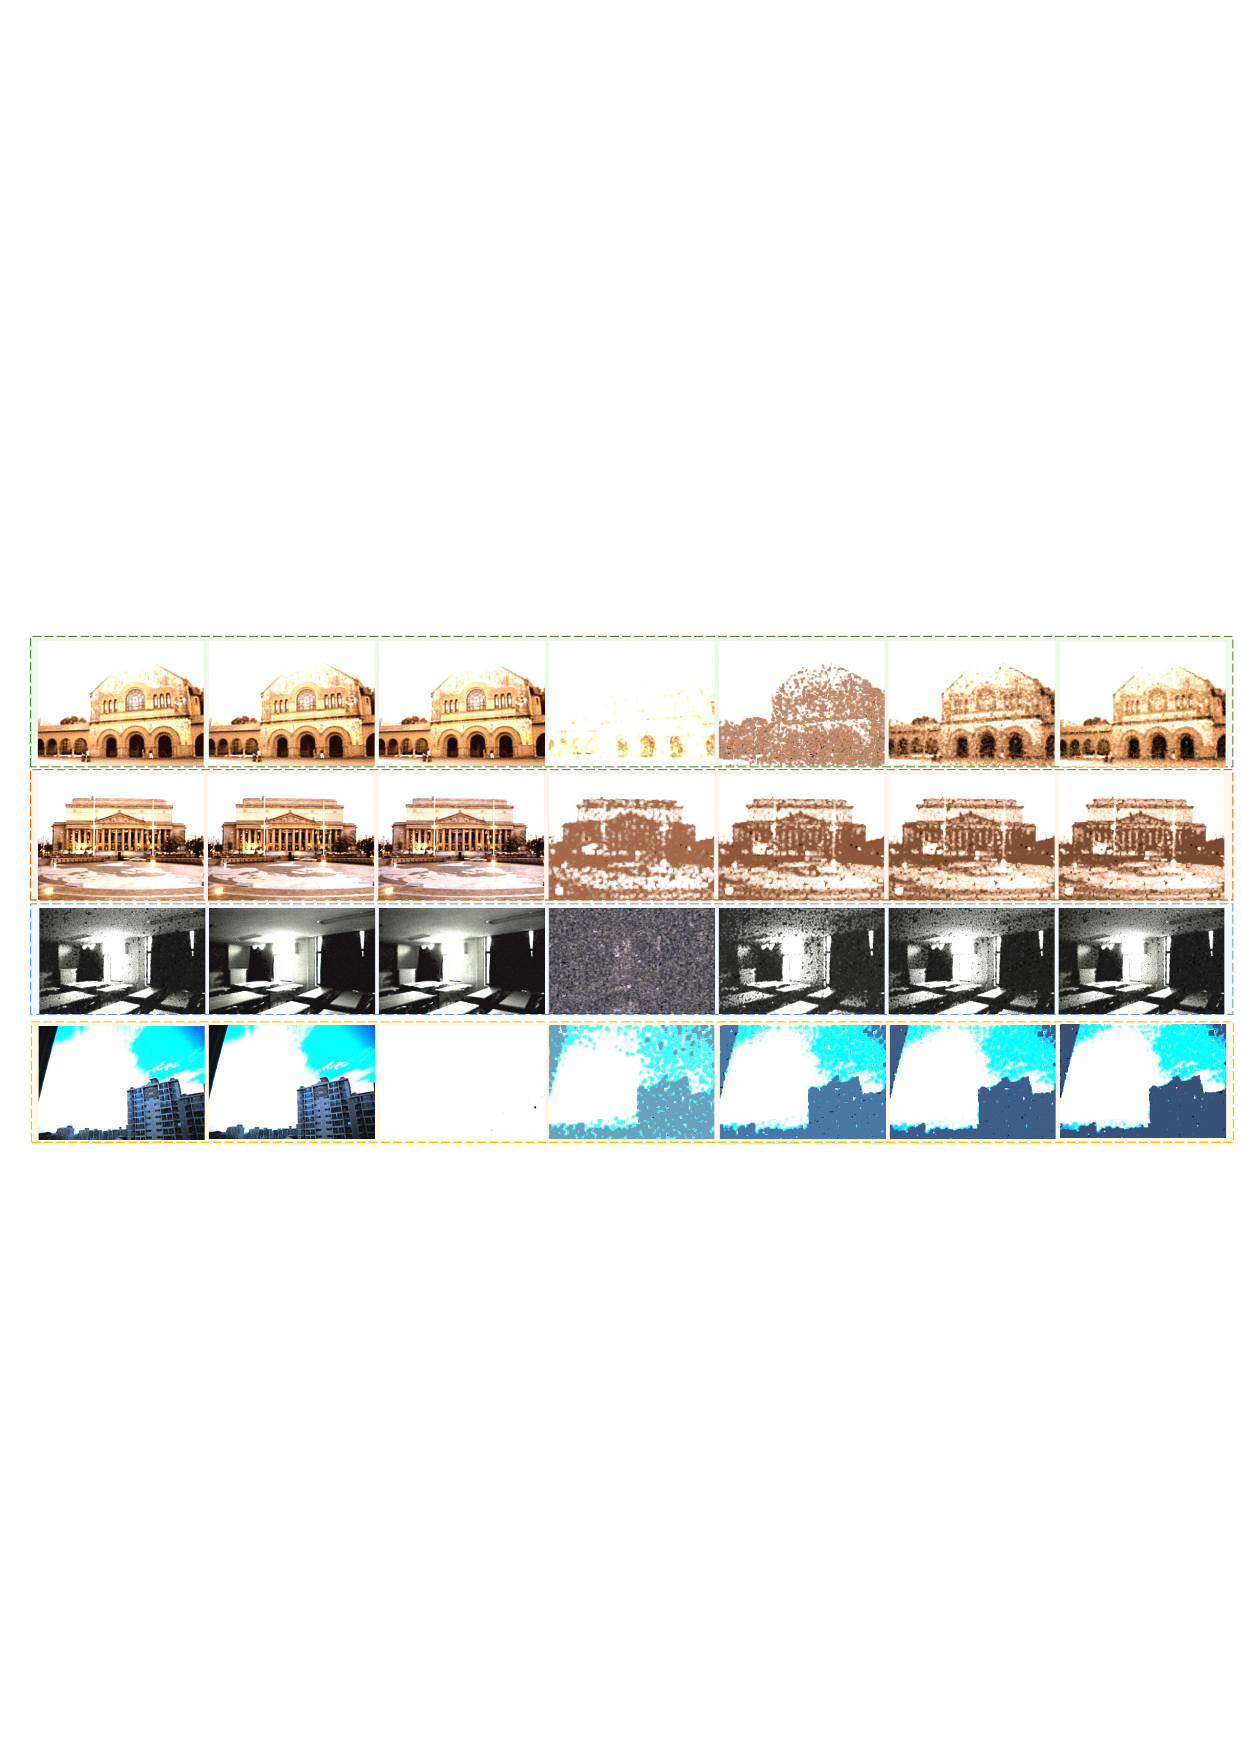}
    \caption{Visual quality comparison about Motivation. All pictures are the process of selecting and optimizing the parameters of the pre-trained model. During the iterative optimization process, the method of optimizing model parameters often suddenly collapses at one point in time, and the image quality deteriorates significantly thereafter.}
    \label{fig:supp_optim}
    \vspace{-0.3cm}
\end{figure*}

\begin{figure*}[t]
    \centering
    \includegraphics[width=0.85\linewidth]{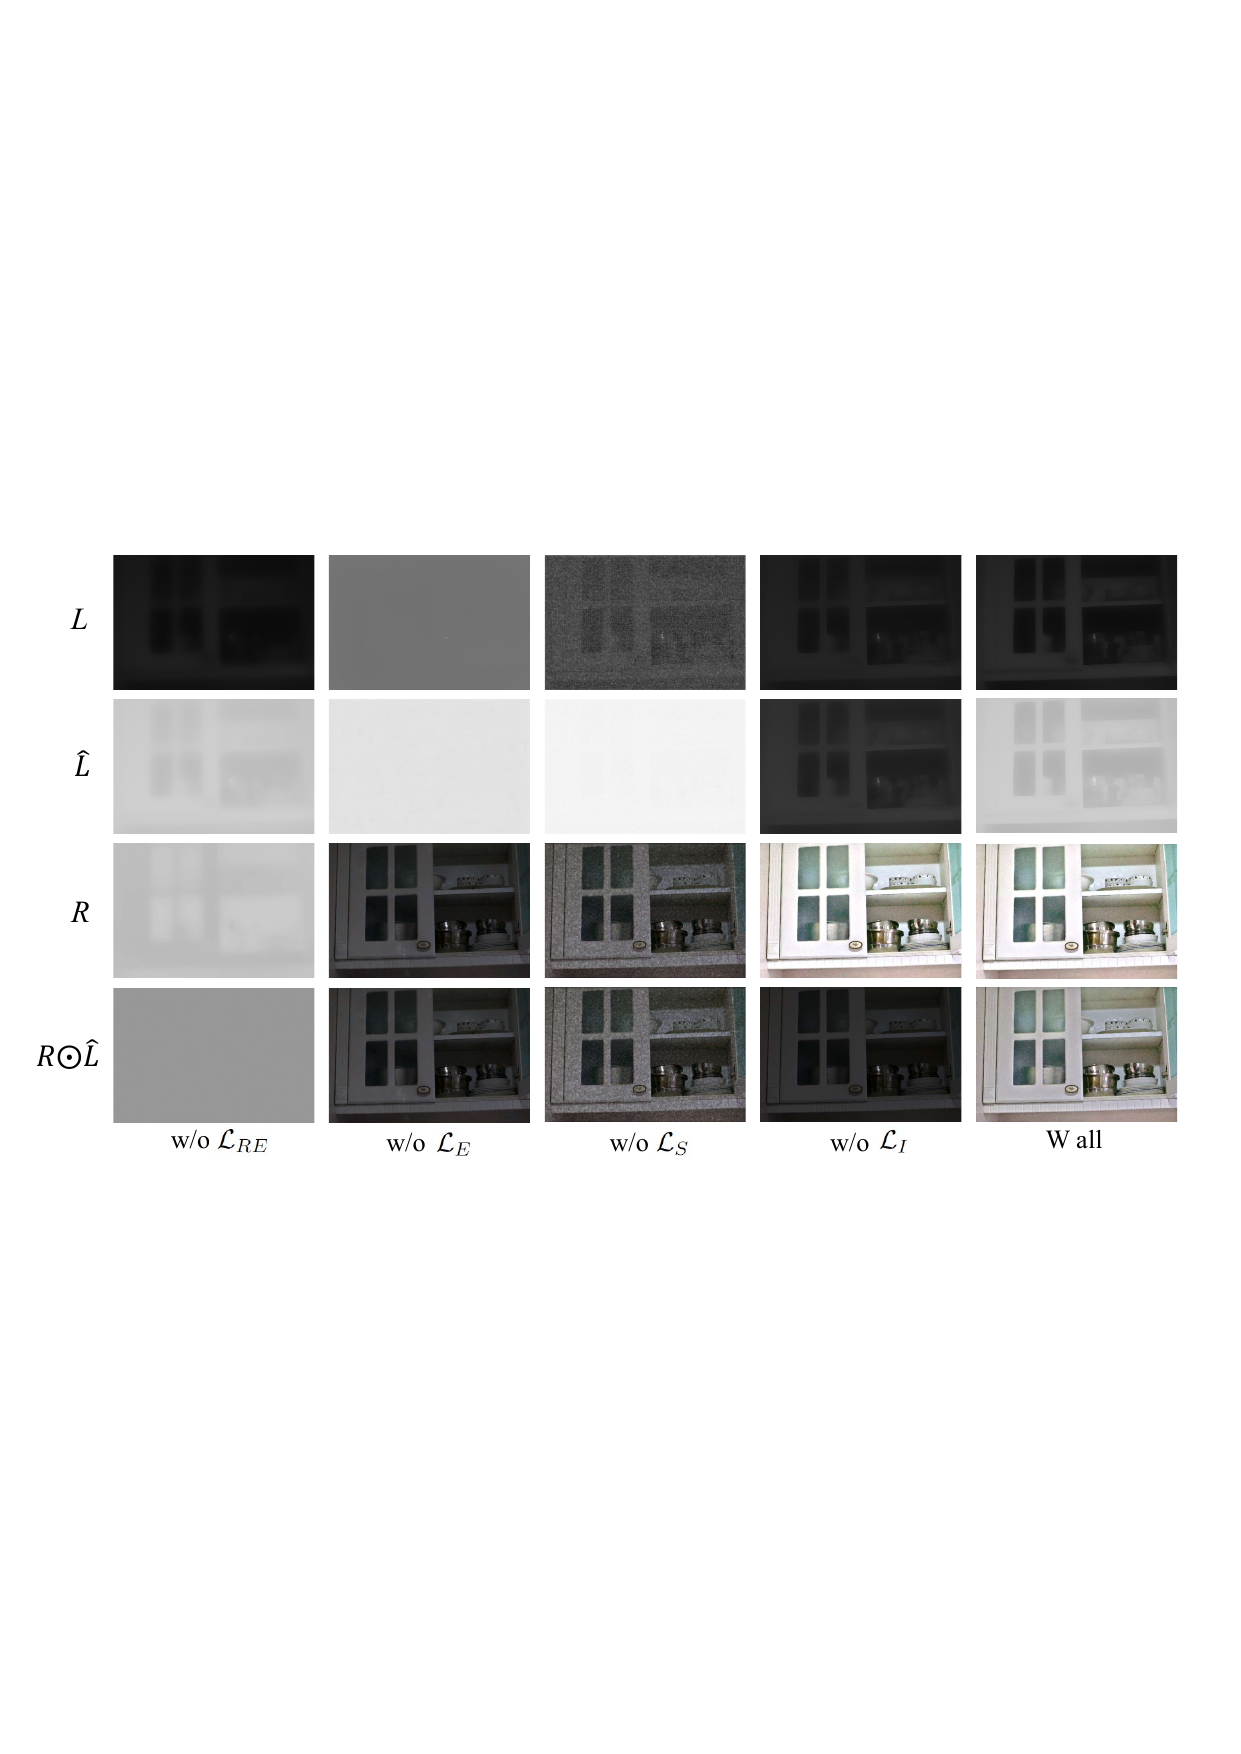}
    \caption{Visual quality comparison about different losses.}
    \label{fig:supp_loss}
    \vspace{-0.3cm}
\end{figure*}

In our framework, the loss components $\mathcal{L}_{RE}$ and $\mathcal{L}_I$ are crucial for image reconstruction and brightness enhancement in low-light enhancement tasks, while $\mathcal{L}_E$ and $\mathcal{L}_S$ contribute to stable Retinex decomposition and improved image quality. Section X details the impact of omitting $\mathcal{L}_E$ and $\mathcal{L}_I$ on model accuracy, and Table~\ref{fig:supp_loss} illustrates the consequences of removing each regularization term. Our findings indicate that the absence of any loss component significantly degrades enhancement performance. Specifically, excluding $\mathcal{L}_{RE}$ hinders the model's ability to accurately represent the original image. Omitting $\mathcal{L}_I$ and $\mathcal{L}_E$ disrupts the light map's enhancement capabilities, and without $\mathcal{L}_S$, the model struggles with efficient noise reduction in extremely dark areas, adversely affecting the fitting speed.
Furthermore, we have analyzed the computational overhead associated with each loss component. As depicted in Table~\ref{supp:tab:time}, the computation of our loss components constitutes approximately 10\% of the total enhancement processing time.

%\section{Application Study}
%$\indent$ In evaluating our proposed method's practical applicability, we conducted tests using two distinct datasets: CODaN and Retina.  CODaN is a 10-class
%dataset containing a training set of 10000 daytime images
%and a test set with 2500 daytime and nighttime images, respectively. We validate models on the daytime test set and
%evaluate them on the nighttime test set. Here we use the weights (resnet50) officially provided by CODaN to evaluate the effects of different low-light enhancement methods. Conversely, Retina, a dataset dedicated to ophthalmological research, facilitates an analysis in a medical context. 
%\input{sec/supp/table_appli}
%Figures X and X in Table Y provide a comparative visualization of the results on CODaN and XXX, respectively. Notably, our approach demonstrates remarkable generalization capabilities, maintaining high-quality visual results across diverse data processing pipelines.

\section{More Visual Comparisons}
$\indent$Here we compare our method with all the methods mentioned in our paper (i.e. all the supervised methods mentioned in our paper (RetinexNet ~\cite{Supervised_2018Retinexnet}, KinD++ ~\cite{Supervised_zhang2021kindpp}, and SNR ~\cite{Supervised_xu2022snr}) with all of their released pre-trained models and all the unsupervised methods mentioned in our paper (DUNP ~\cite{Zeroshot_liang2022dunp}, GDP ~\cite{Zeroshot_fei2023gdp}, Zero-DCE++ ~\cite{UnSupervised_guo2020zerodce}, SCL-LLE ~\cite{UnSupervised_liang2022scllle}, RUAS ~\cite{UnSupervised_liu2021ruas}, EnlightGAN ~\cite{UnSupervised_jiang2021enlightengan},  SGZ ~\cite{UnSupervised_zheng2022SGZ}, NeRCo~\cite{UnSupervised_yang2023nerco}, SCI ~\cite{UnSupervised_ma2022sci} and Ours)) on the every test datasets.

Figs.~\ref{fig:supp_compare_1},~\ref{fig:supp_compare_2}, ~\ref{fig:supp_compare_3} show more visual comparisons between the results generated by our methods and the compared methods. By comparison, our model realizes the best visual quality with prominent contrast and vivid colors, while restoring intricate details. This is very surprising especially since most other methods use large amounts of low-light image data and require lengthy training or inference processes.

\begin{figure*}[t]
    \centering
    \includegraphics[width=\linewidth]{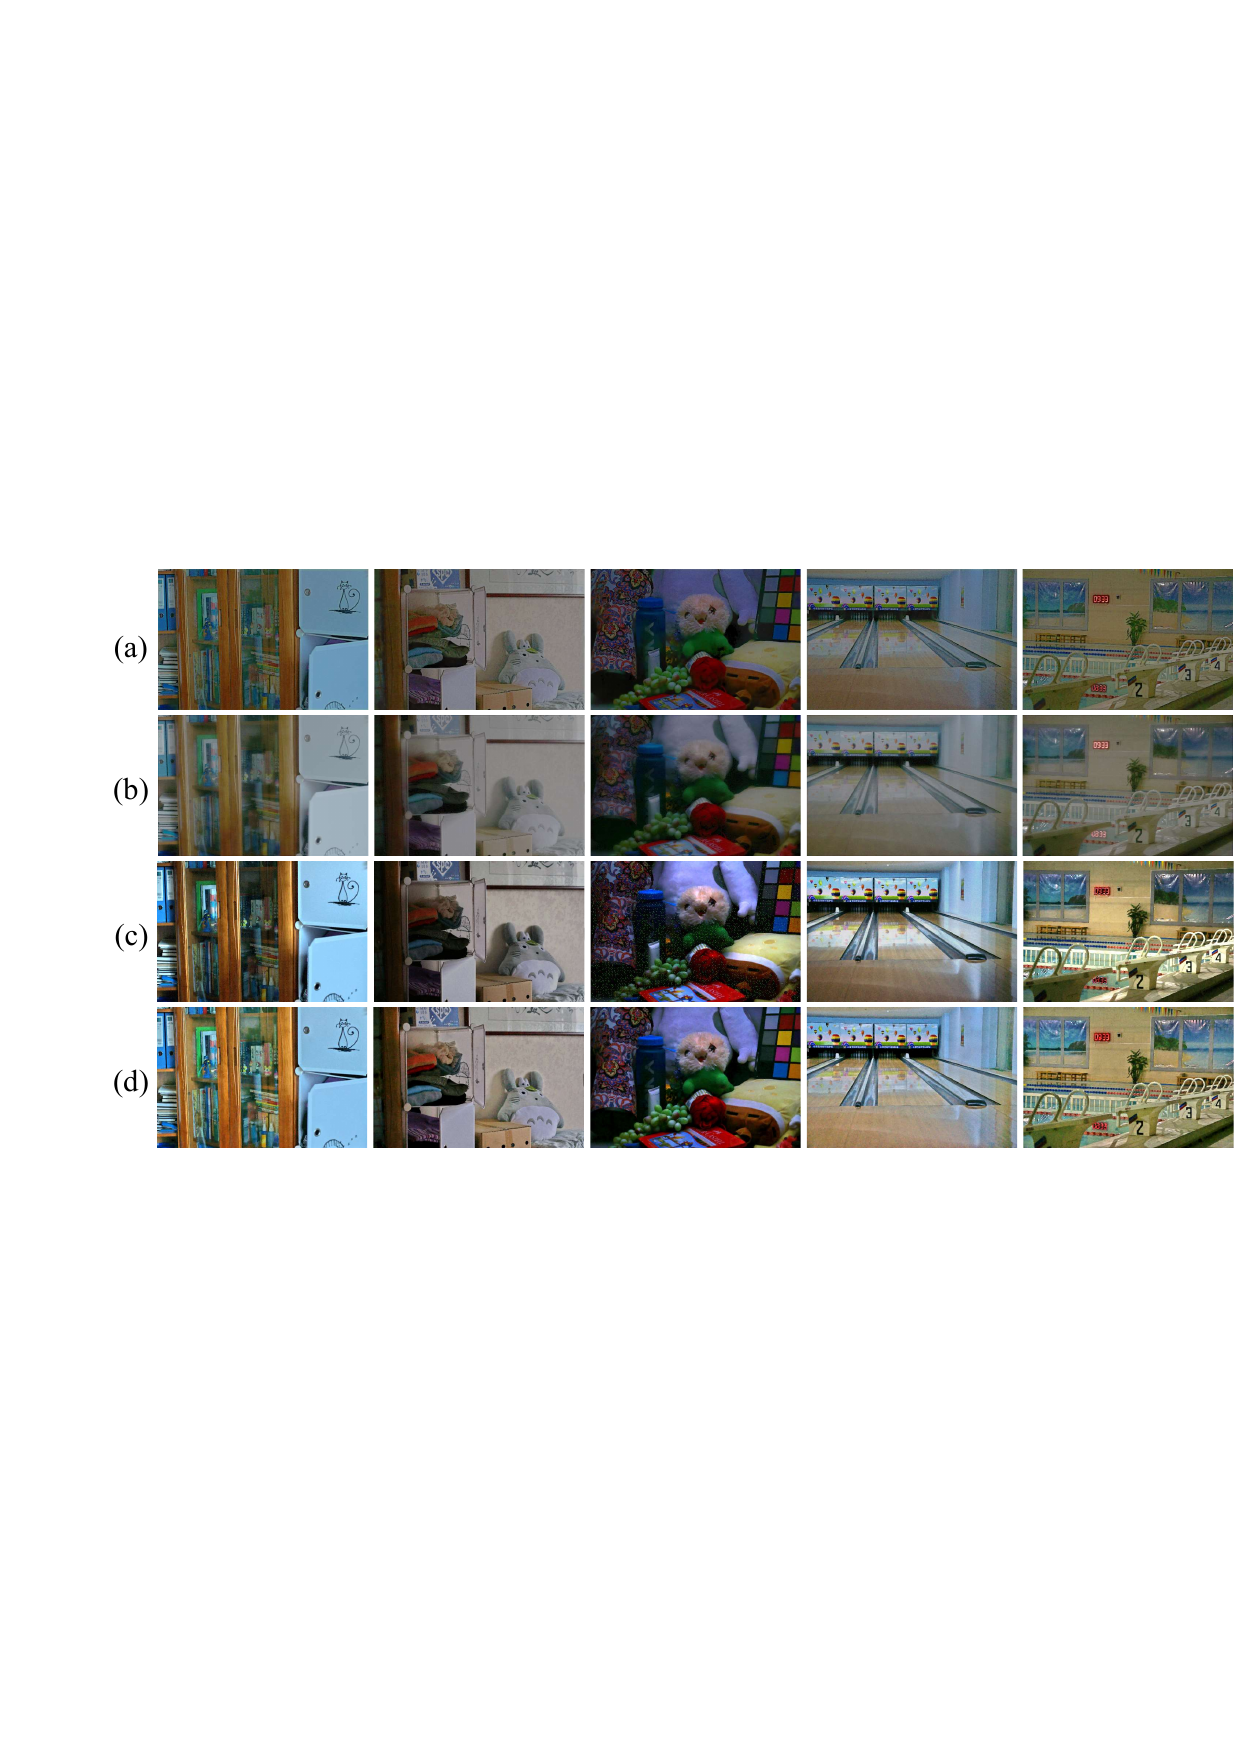}
    \caption{Visual quality comparison of different pre-training models. (a) is DCGAN, (b) is EAGAN, (c) is VAE, and (d) is VQVAE-2, which is the pre-training model used in the proposed method.}
    \label{fig:supp_pretrains}
\end{figure*}

\begin{figure*}[h]
    \centering
    \includegraphics[width=\linewidth]{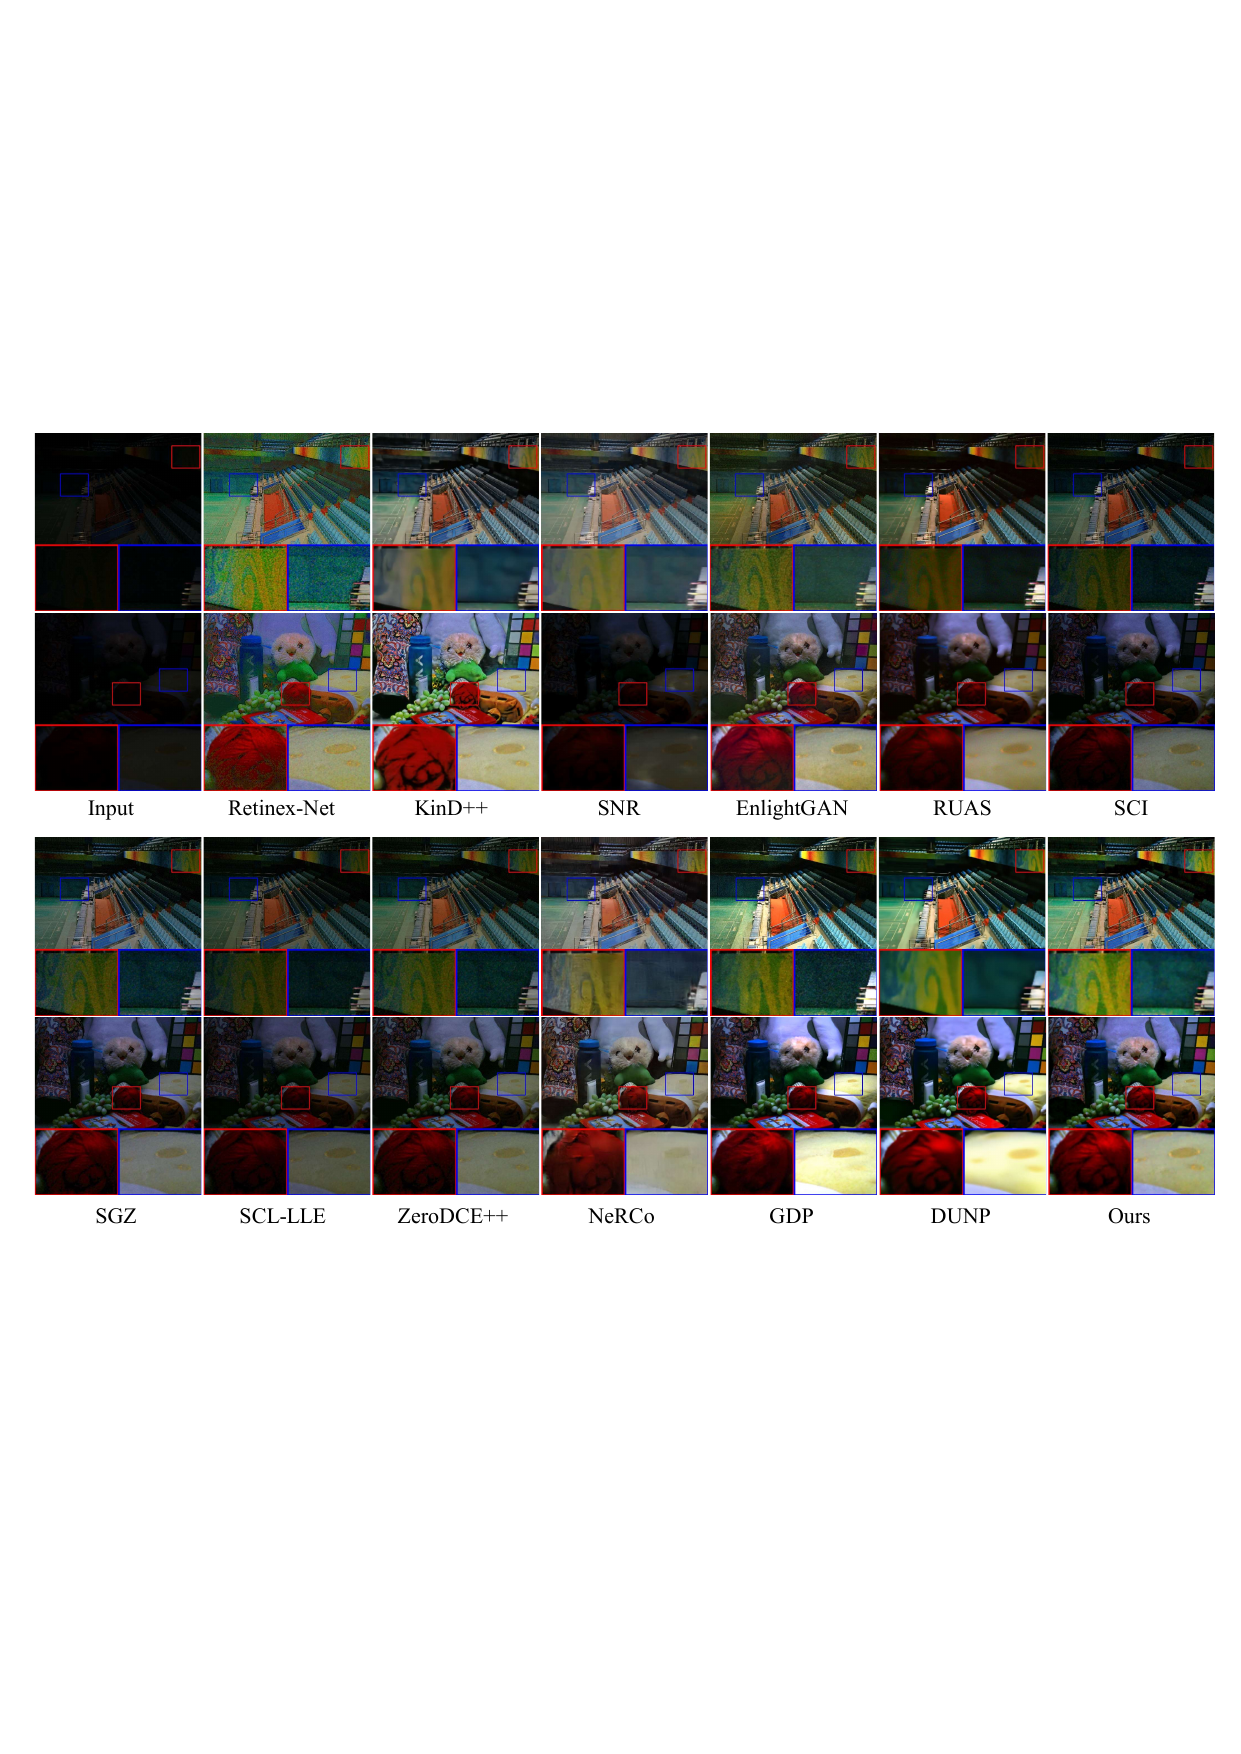}
    \caption{Visual quality comparison.}
    \label{fig:supp_compare_1}
    \vspace{-0.3cm}
\end{figure*}

\begin{figure*}[h]
    \centering
    \vspace{-0.3cm}
    \includegraphics[width=\linewidth]{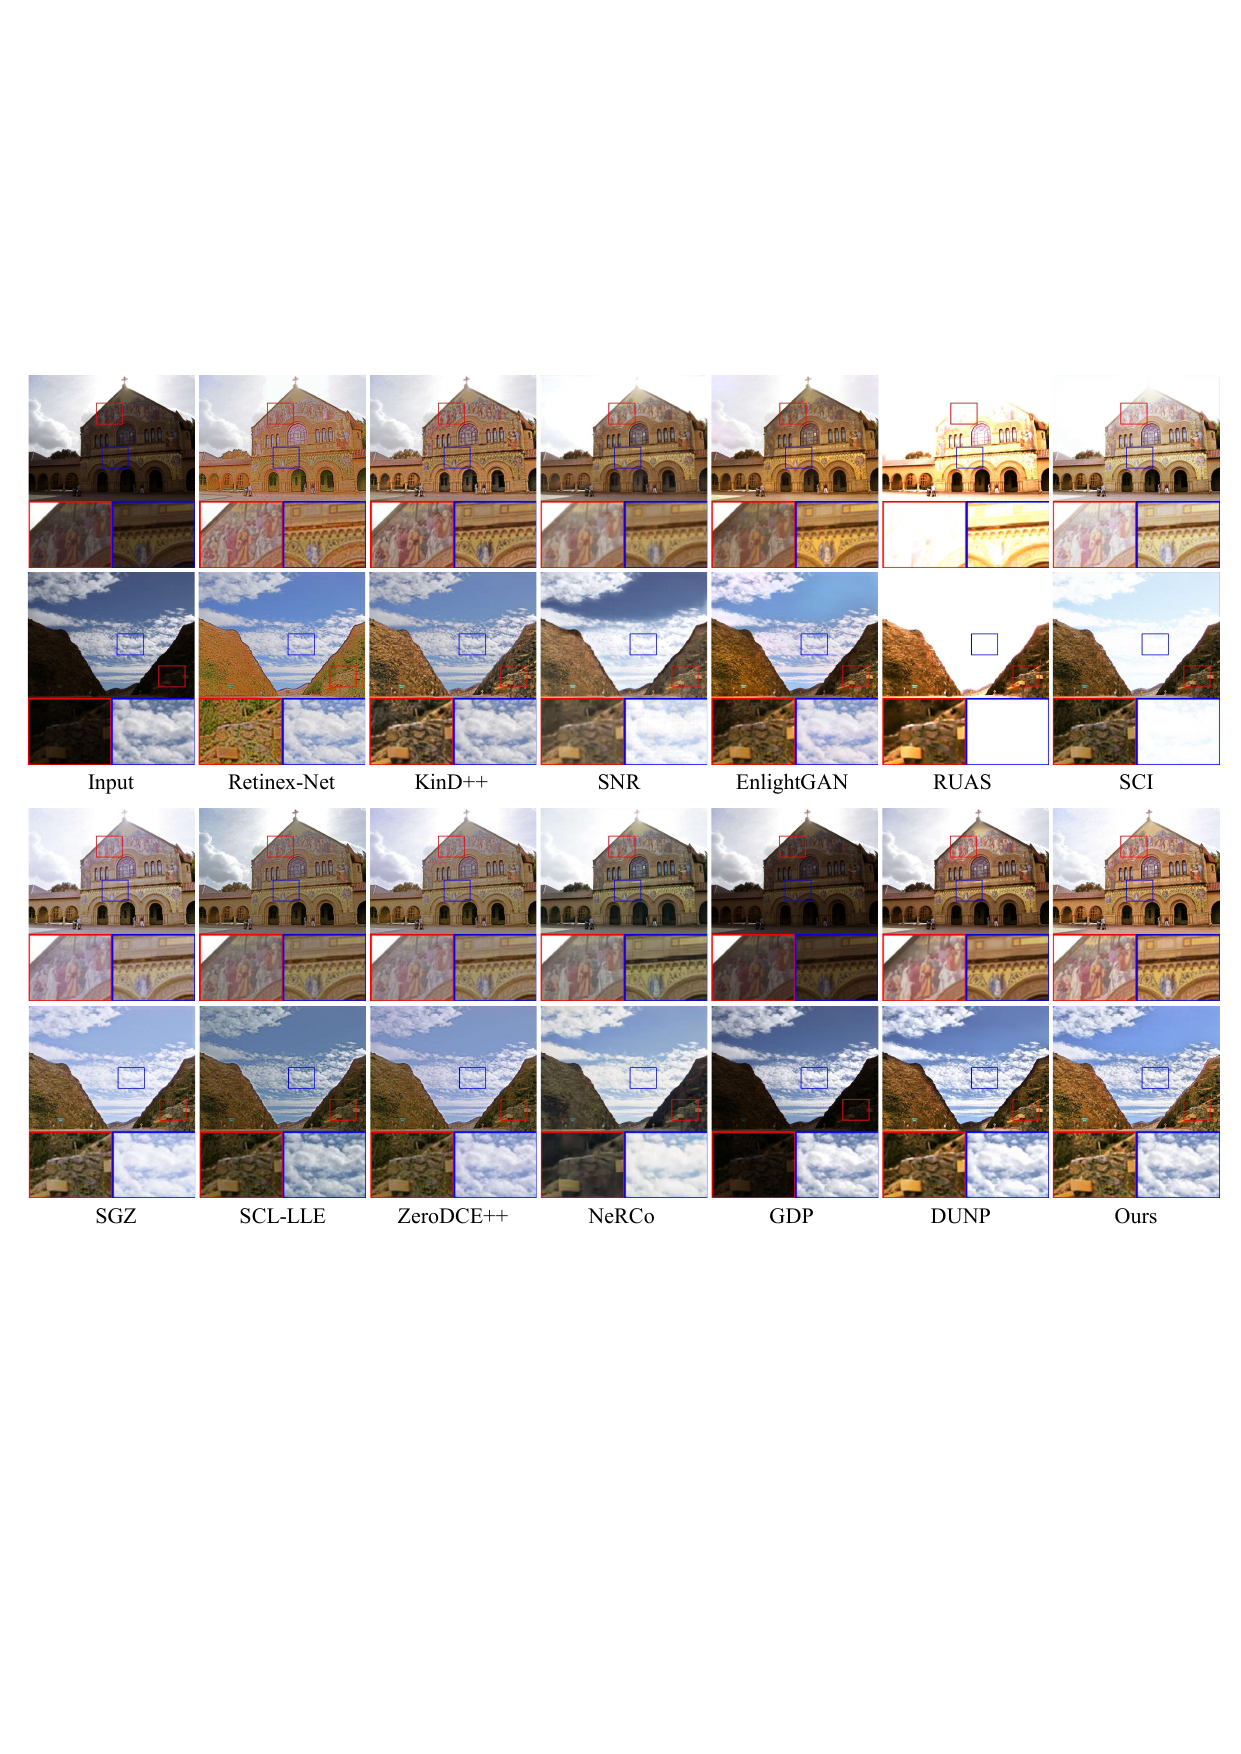}
    \caption{Visual quality comparison.}
    \label{fig:supp_compare_2}
    \vspace{-0.3cm}
\end{figure*}

\begin{figure*}[h]
    \centering
    \vspace{-0.3cm}
    \includegraphics[width=\linewidth]{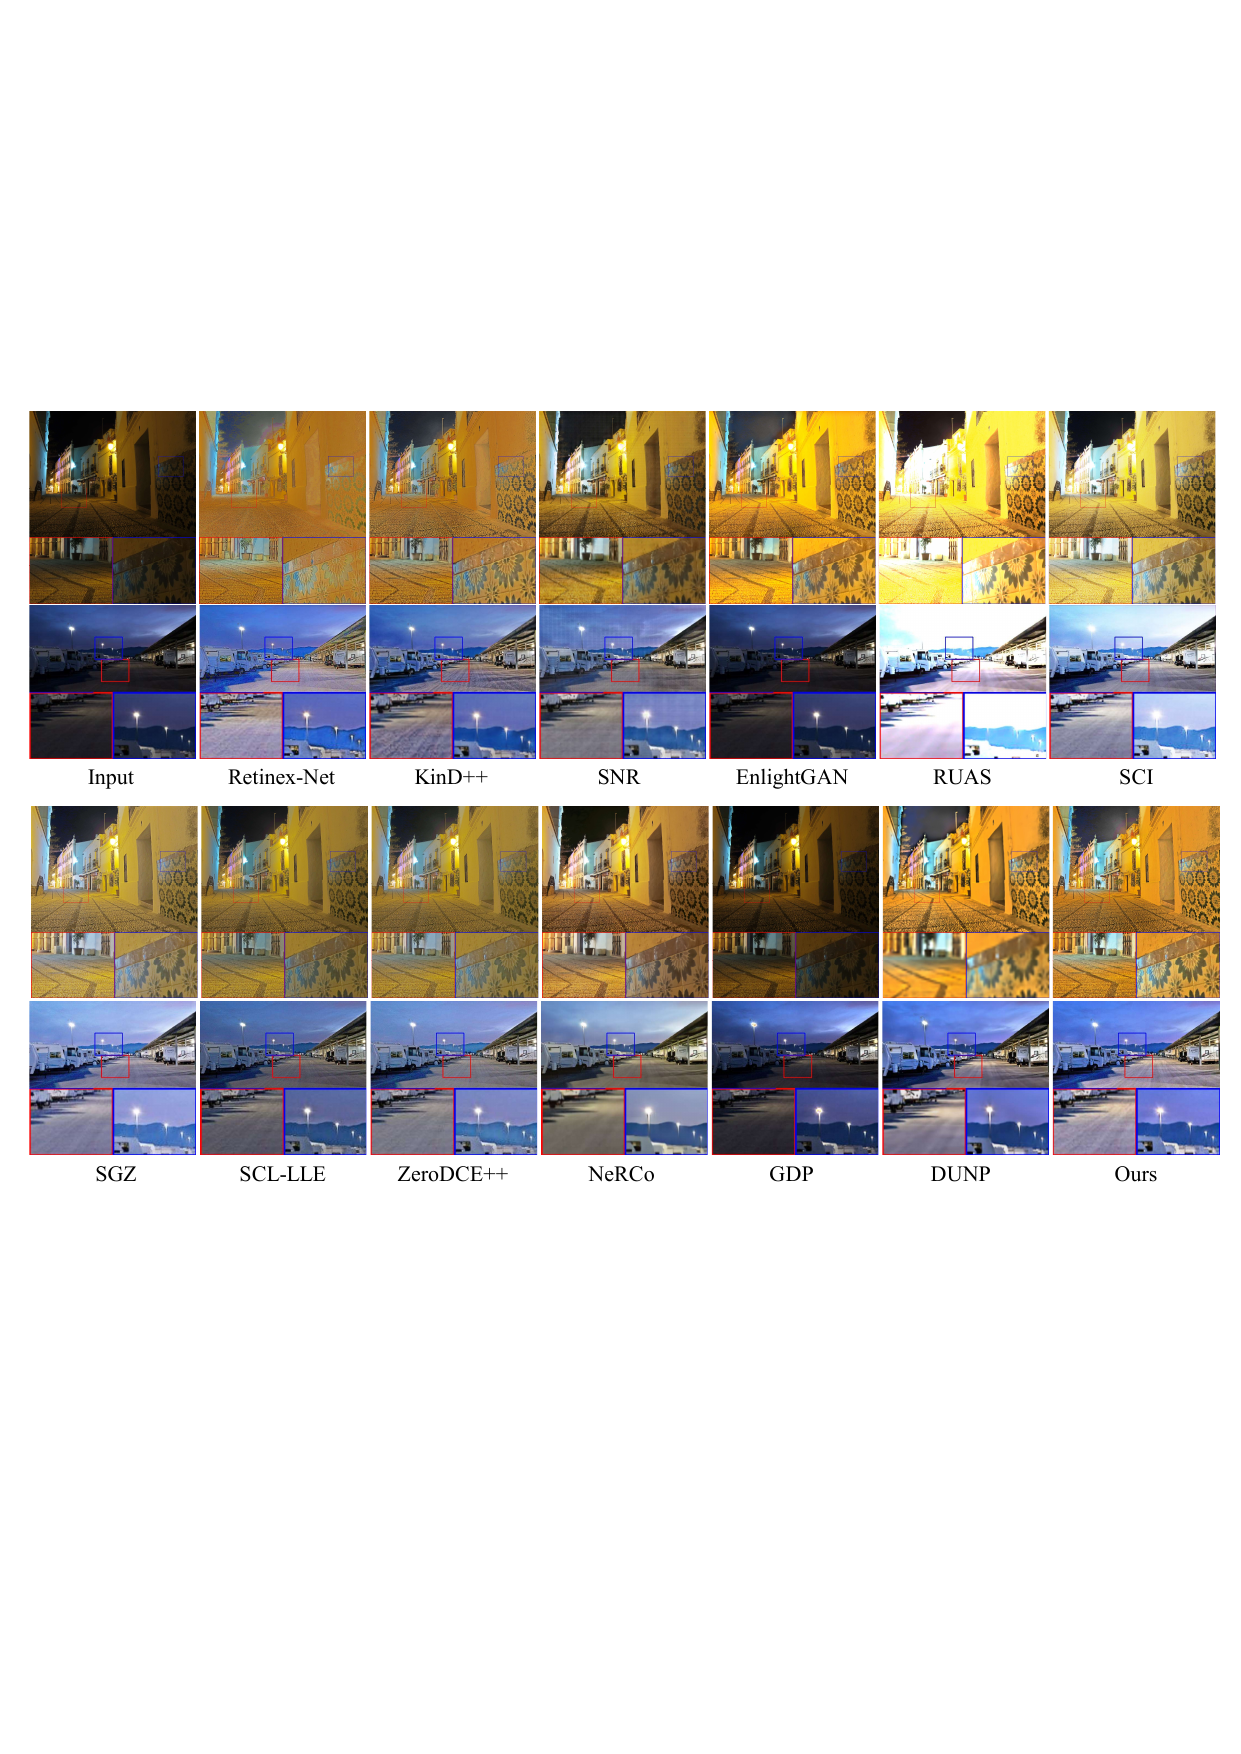}
    \caption{Visual quality comparison.}
    \label{fig:supp_compare_3}
    \vspace{-0.3cm}
\end{figure*}
