# Supplementary material for: Seed Optimization with Frozen Generator for Superior Zero-shot Low-light Enhancement
Source: arXiv:2402.09694 source file (2024-02-15)
Supplement: Supplementary file 3 [file table_pretrain.tex]

\begin{table}[h]
\centering
\resizebox{\columnwidth}{!}{
\begin{tabular}{lcccc}
\hline
\multicolumn{1}{c}{Method} & DCGAN       & EAGAN    & VAE     & VQVAE-2       \\ \hline
Dataset                    & Imagenet-1K & Imagenet-1K & COCO    & Imagenet+FFHQ \\
PSNR↑                       & 16.09       & 16.94    & 17.19   & 18.10         \\
SSIM↓                       & 0.69        & 0.74     & 0.72    & 0.75          \\
Iteration                  & 4000        & 3000     & 5000    & 2500          \\
Runtime                    & 0.06259     & 0.18580  & 0.01035 & 0.00813       \\
Totaltime                  & 250.8       & 557.4    & 51.75   & 20.3       \\ \hline
\end{tabular}
}
\caption{Training details and effects used by different pretrained generators.}
\label{supp:tab:pretrain}
\end{table}
