# Supplementary material for: Seed Optimization with Frozen Generator for Superior Zero-shot Low-light Enhancement
Source: arXiv:2402.09694 source file (2024-02-15)
Supplement: Supplementary file 4 [file table_time.tex]

\begin{table}[h]
\centering
\resizebox{0.5\columnwidth}{!}{
\begin{tabular}{lc}
\hline
\multicolumn{1}{c}{Method} &Time   \\ \hline
$\mathcal{L}_S$                   & 1.548s \\
$\mathcal{L}_E$                       & 0.194s \\
$\mathcal{L}_{RE}$                       & 0.254s \\
$\mathcal{L}_I$                       & 0.155s \\
other process              & 18.174 \\
totaltime                  & 20.325 \\ \hline
\end{tabular}
}
\caption{Analysis of the time occupied by each loss during the execution of the proposed method.}
\label{supp:tab:time}
\end{table}
